# Supplementary material for: Learning Interpretable BEV Based VIO without Deep Neural Networks
Source: arXiv:2109.12292 source file (2022-09-17)
Supplement: Supplementary file 1 [file pseudocode_Loc.tex]

\begin{figure*}[]
 \begin{minipage}[t]{\textwidth}
 \vspace{-30pt}
\begin{algorithm}[H]
	%\textsl{}\setstretch{1.8}

	\caption{BEVO For Localization (BEVO+)}
	\label{algo:loc}
	\begin{algorithmic}[1]
		\REQUIRE $image_{t-1}, image_{t}, imu \_ data, drone\_ map,$
		$x_{t-1}, y_{t-1}, yaw_{t-1} $
		\ENSURE $ x_t, y_t, yaw_t$
		\STATE $[\Delta x_{t-1}, \Delta y_{t-1}, \Delta yaw_{t-1}] \leftarrow$ \textbf{BEVO(}$image_{t-1}$, $image_{t}$, $imu\_ data$ \textbf{)}
		\STATE $[x_t^{*}, y_t^{*}, yaw_t^{*}] \leftarrow [x_{t-1}+\Delta x_{t-1}, y_{t-1}+\Delta y_{t-1}, yaw_{t-1}+\Delta yaw_{t-1}]$
		\STATE Load bev image of $image_{t}$ from BEVO as $image_t^{b}$.
		\STATE $image_t^{*} \leftarrow $ \textbf{CropInDroneMap(} $x_t^{*}, y_t^{*}, yaw_t^{*}$ \textbf{)} 
		\STATE $[\Delta x_t^{'}, \Delta y_t^{'}, \Delta yaw_t^{'}] \leftarrow $ \textbf{DPC(} $image_t^{b}$, $image_t^{*}$ \textbf{)} 
		\STATE $[x_{t\_ measure}, y_{t\_ measure}, yaw_{t\_ measure}] \leftarrow [x_t^{*}+\Delta x_t^{'}, y_t^{*}+\Delta y_t^{'}, yaw_t^{*}+\Delta yaw_t^{'}]$
		\STATE $[x_t, y_t, yaw_t] \leftarrow $ \textbf{UKF\_ ForLocalization(}$[x_{t-1},y_{t-1},yaw_{t-1}],$\par
		\hskip\algorithmicindent$[\Delta x_{t-1}, \Delta y_{t-1},\Delta yaw_{t-1}],$ \par
		\hskip\algorithmicindent$[x_{t\_ measure},y_{t\_ measure},yaw_{t\_ measure}]$\textbf{)}
		\RETURN $x_t, y_t, yaw_t$
	\end{algorithmic}  
\end{algorithm}
\end{minipage}
\vspace{5pt}
\begin{minipage}[h]{\textwidth}
\vspace{-10pt}
\begin{algorithm}[H]
	%\textsl{}\setstretch{1.8}

	\caption{UKF\_ForLocalization}
	\label{algo:loc_ukf}
	\begin{algorithmic}[1]
		\REQUIRE $ [x_{t-1},y_{t-1},yaw_{t-1}],[\Delta x_{t-1\_ odom}, \Delta y_{t-1\_ odom}, \Delta yaw_{t-1\_ odom}], $\par
		\hskip\algorithmicindent $[x_{t\_ measure},y_{t\_ measure},yaw_{t\_ measure}]$
		\ENSURE $[x_t, y_t, yaw_t]$
		\STATE \textbf{Load $\mu _{t-1},\sigma _{t-1}$ into this recursion.}
		\STATE $X_{t-1} \leftarrow$ Sampling($[x_{t-1},y_{t-1},yaw_{t-1}],\sigma_{t-1} $)
		\STATE $\bar{X}_{t}^{*} \leftarrow $ \textbf{MotionModel(}$X_{t-1},[\Delta x_{t-1\_ odom}, \Delta y_{t-1\_ odom}, \Delta yaw_{t-1\_ odom}]$  \textbf{)}
		\STATE $\bar{\mu}_{t} \leftarrow $ WeightedAverage($\bar{X}_t^{*}$)
		\STATE $\bar{\sigma}_t \leftarrow $ WeightedAverage[$(\bar{X}_{t}^{*}-\bar{\mu}_{t})(\bar{X}_{t}^{*}-\bar{\mu}_{t})^{T}$] + Motion Noise $O_t$
		\STATE $\bar{X}_t \leftarrow $ Sampling($\bar{\mu}_t$, $\bar{\sigma}_t$)
		\STATE $\bar{Z}_t \leftarrow $ \textbf{MeasurementModel(}$\bar{X}_t$\textbf{)}
		\STATE $\bar{M_t} \leftarrow $ WeightedAverage($\bar{Z}_t$)
		\STATE $\bar{\sum}_t \leftarrow $ WeightedAverage[$(\bar{Z}_{t}-\bar{M}_{t})(\bar{Z}_{t}-\bar{M}_{t})^{T}$] + Measurement Noise $Q_t$
		\STATE $\bar{\sum}_t^{X,Z} \leftarrow $ WeightedAverage[$(\bar{X}_{t}^{i}-\bar{\mu}_{t})(\bar{Z}_{t}^{i}-\bar{M}_{t})^{T}$]
		\STATE $K_t \leftarrow \bar{\sum}_t^{X,Z} \bar{\sum}_t^{-1} $
		\STATE $Z_t \leftarrow [x_{t\_ measure},y_{t\_ measure},yaw_{t\_ measure}]$
		\STATE $\mu _t \leftarrow \bar{\mu}_t+K_t(Z_t-\bar{M}_t)$
		\STATE $\sigma _t \leftarrow \bar{\sigma}_t+K_t\bar{\sum}_tK_t^{-1}$
		\STATE $[x_t,y_t,yaw_t] \leftarrow \mu _t$
		\RETURN $x_t,y_t,yaw_t$
	\end{algorithmic}  
\end{algorithm}
\end{minipage}
\end{figure*}
