# Supplementary material for: Learning Interpretable BEV Based VIO without Deep Neural Networks
Source: arXiv:2109.12292 source file (2022-09-17)
Supplement: Supplementary file 2 [file BEVO_pseudo.tex]

\begin{algorithm}[t]
	%\textsl{}\setstretch{1.8}
	\algsetup{linenosize=\tiny}
	\footnotesize

	\caption{BEVO}
	\label{pseudocode:BEVO}
	\begin{algorithmic}[1]
		\REQUIRE $image_{t-1}, image_{t}, imu \_ data$, Ground Truth:$\textbf{t}^{*}_{t}, \theta^{*}_{t}$
		\ENSURE 2D translation: $\textbf{t}_{t}$, pitch: $\alpha_{t}$, roll: $\beta_{t}$, yaw: $\theta_{t}$
		\STATE \textbf{Load $\alpha_{t-1},\beta_{t-1}$ from last recursion of BEVO into this recursion.}
		\STATE \textbf{Load $\omega_{\alpha_{t-1}}, \omega_{\beta{t-1}}$ from $imu\_data$}
		\STATE \textbf{Load $acc_{t}^{x}, acc_{t}^{y}, acc_{t}^{z}$ from $imu\_data$}
		\STATE \textbf{Load $\Delta t$ from $imu\_data$}
		\STATE $[\Delta \alpha_{t-1},\Delta\beta_{t-1}] \leftarrow [\omega_{\alpha_{t-1}}, \omega_{\beta{t-1}}]\times \Delta t$
		\STATE $\alpha\_measure_t \leftarrow -arctan(acc_t^{x}/\sqrt{{acc^{y}_t}^2+{acc_t^{z}}^2})$
		\STATE $\beta\_measure_t \leftarrow arctan(acc_t^{y}/acc_t^{z})$
		\STATE $[\alpha_{t}, \beta_{t}] \leftarrow \textbf{UKF(} [\alpha_{t-1}, \beta_{t-1}],[\Delta \alpha_{t-1}, \Delta \beta_{t-1}],[\alpha\_measure_{t},\beta\_measure_{t}]\textbf{)}$
		\STATE $image_{t-1}^{bev} \leftarrow \textbf{BEVProjection(} image_{t-1}, \alpha_{t-1}, \beta_{t-1} \textbf{)}$
		\STATE $image_{t}^{bev} \leftarrow \textbf{BEVProjection(} image_{t}, \alpha_{t}, \beta_{t} \textbf{)}$
		\STATE $[\textbf{t}_{t}, \theta_{t}] \leftarrow \textbf{DPC(} image_{t-1}^b, image_{t}^b$ \textbf{)}
		\STATE \textbf{Loss} $\mathcal{L}([\textbf{t}^{*}_{t},\theta^{*}_{t}],[\textbf{t}_{t}, \theta_{t}])$
		\STATE \textbf{Backward}
		\RETURN $ \textbf{t}_{t}, \theta_{t}, \alpha_{t}, \beta_{t}$
	\end{algorithmic}  
\end{algorithm}
