# Supplementary material for: Learning Interpretable BEV Based VIO without Deep Neural Networks
Source: arXiv:2109.12292 source file (2022-09-17)
Supplement: Supplementary file 3 [file CUD.tex]

\begin{table}[]
\centering
\caption{Quantitative results on Complex Urban Dataset}
\begin{tabular}{@{}cc|lll|lll@{}}
\toprule
Seq & & \multicolumn{1}{c}{Urban30} & \multicolumn{1}{c}{Urban31} & Urban32 & Urban33 & Urban34 & Urban35 \\ \midrule

\multirow{2}{*}{ORB-M} & $t_{rel}$ & 
17.42 & 16.29 & 19.01 & 18.56 & 18.75 & 16.47 \\
 & $r_{rel}$ & 
4.65 & 6,21 & 5.44 & 4.86 & 6.82 & 5.79 \\

\multirow{2}{*}{BEVO} & $t_{rel}$ & 
0.96 & 0.88 & 0.92 & 0.98 & 1.01 & 0.99 \\
 & $r_{rel}$ & 
1.01 & 1.04 & 0.99 & 1.10 & 1.02 & 0.99 \\ \bottomrule
\end{tabular}
\label{tab:CUD}
\end{table}
