# Supplementary material for: Learning Interpretable BEV Based VIO without Deep Neural Networks
Source: arXiv:2109.12292 source file (2022-09-17)
Supplement: Supplementary file 4 [file pseudocode_UKF.tex]

\begin{algorithm}
	%\textsl{}\setstretch{1.8}

	\caption{Unscented Kalman Filter (UKF)}
	\label{algo:UKF}
	\begin{algorithmic}[1]
		\REQUIRE $ x_{t-1},\Delta x_{t-1}, x\_measure_{t}$
		\ENSURE $x_t$
		\STATE \textbf{Load $\mu _{t-1},\sigma _{t-1}$ into this recursion.}
		\STATE $X_{t-1} \leftarrow$ Sampling($[x_{t-1}],\sigma_{t-1} $)
		\STATE $\bar{X}_{t}^{*} \leftarrow $ \textbf{MotionModel(}$X_{t-1},[\Delta x_{t-1}]$  \textbf{)}
		\STATE $\bar{\mu}_{t} \leftarrow $ WeightedAverage($\bar{X}_t^{*}$)
		\STATE $\bar{\sigma}_t \leftarrow $ WeightedAverage[$(\bar{X}_{t}^{*}-\bar{\mu}_{t})(\bar{X}_{t}^{*}-\bar{\mu}_{t})^{T}$] + Motion Noise $O_t$
		\STATE $\bar{X}_t \leftarrow $ Sampling($\bar{\mu}_t$, $\bar{\sigma}_t$)
		\STATE $\bar{Z}_t \leftarrow $ \textbf{MeasurementModel(}$\bar{X}_t$\textbf{)}
		\STATE $\bar{M_t} \leftarrow $ WeightedAverage($\bar{Z}_t$)
		\STATE $\bar{\sum}_t \leftarrow $ WeightedAverage[$(\bar{Z}_{t}-\bar{M}_{t})(\bar{Z}_{t}-\bar{M}_{t})^{T}$] + Measurement Noise $Q_t$
		\STATE $\bar{\sum}_t^{X,Z} \leftarrow $ WeightedAverage[$(\bar{X}_{t}^{i}-\bar{\mu}_{t})(\bar{Z}_{t}^{i}-\bar{M}_{t})^{T}$]
		\STATE $K_t \leftarrow \bar{\sum}_t^{X,Z} \bar{\sum}_t^{-1} $
		\STATE $Z_t \leftarrow [x\_measure_t]$
		\STATE $\mu _t \leftarrow \bar{\mu}_t+K_t(Z_t-\bar{M}_t)$
		\STATE $\sigma _t \leftarrow \bar{\sigma}_t+K_t\bar{\sum}_tK_t^{-1}$
		\STATE $x_t \leftarrow \mu _t$
		\RETURN $x_t$
	\end{algorithmic}  
\end{algorithm}
