# Supplementary material for: Learning Interpretable BEV Based VIO without Deep Neural Networks
Source: arXiv:2109.12292 source file (2022-09-17)
Supplement: Supplementary file 5 [file runtime.tex]

\begin{table}[]
\centering
\label{tab:runtime}
\caption{The relationships between BEV size, accuracy, runtime, and memory statistic.}
\begin{tabular}{@{}clllllll@{}}
\toprule
Indicators  & \multicolumn{7}{c}{Performance}                \\ \midrule
BEV Size & \multicolumn{1}{c}{80} & \multicolumn{1}{c}{90} & \multicolumn{1}{c}{100} & \multicolumn{1}{c}{110} & 120 & 200 & 240 \\
$t_{rel}$           & 2.01 & 1.56 & 1.22 & 1.20 & 1.16 & 1.01 & 1.00 \\
$r_{rel}$           & 1.31 & 1.12 & 1.05 & 1.05 & 1.01 & 0.79 & 0.77 \\
Runtime(ms) & 18   & 18   & 21   & 30   & 43   & 96   & 126  \\
Memory (GB) & 0.45 & 0.46 & 0.51 & 0.62 & 0.77 & 2.04 & 2.99 \\ \bottomrule
\label{tab:runtime}
\end{tabular}
\label{tab:runtime}
\end{table}
